# Supplementary material for: Konzept f\"ur Bildanalysen in Hochdurchsatz-Systemen am Beispiel des Zebrab\"arblings
Source: arXiv:1705.02962 source file (2017-04-26)
Supplement: Supplementary file 1 [file appendix.tex]

\begin{appendix}

\chapter{Wichtige Symbole und Bezeichnungen}
Beim hier gew\"{a}hlten Bezeichnungsapparat wurde ein Kompromiss zwischen einheitlichen und
durchg\"{a}ngigen Bezeichnungen einerseits sowie literaturkonformen und einfachen Bezeichnungen
andererseits gew\"{a}hlt.

Anmerkungen:
\begin{myaufz}
 \item  Das Symbol $\hat{x}$ zeigt immer an, dass es sich um eine Sch\"{a}tzung
 f\"{u}r $x$ handelt.
 \item Ein $\overline{x}$ bedeutet in der Statistik einen Mittelwert f\"{u}r das Symbol $x$, in der
 Logik eine Negation.
 \item Ein $\dot{x}$ kennzeichnet eine Ableitung des Merkmals $x$ nach der Zeit $t$.
 \item Sofern nicht anderweitig vermerkt, kennzeichnen fett gedruckte Gro{\ss}buchstaben Matrizen, fett
 gedruckte Kleinbuchstaben Vektoren und normal gesetzte Zeichen in Symbolen skalare Werte.
 \item Optimale L\"{o}sungen f\"{u}r ein Symbol $x$ werden durch $x_{opt}$ bezeichnet.
 \item Mengen werden durch das Aufz\"{a}hlen von Elementen mit beispielsweise $y \in \{0,1\}$, durch die Angabe von
 offenen Intervallen $y \in (0,1)$ (alle Werte zwischen Null und Eins geh\"{o}ren zur Menge) oder geschlossenen Intervallen $y \in [0,1]$
 (Werte Null, Eins und alle Werte dazwischen geh\"{o}ren zur Menge) angegeben.
\end{myaufz}
\vspace{1cm}
% \tablehead    {\hline Symbol&Bezeichnung \\ \hline}
% \tabletail    {\hline}
% \tablelasttail{\hline}
% \begin{supertabular}{|p{.15\textwidth}||p{.79\textwidth}|}
 \noindent
 \newpage
 \begin{tabular}{p{.15\columnwidth}p{.79\columnwidth}}
 \hline
 Symbol&Bezeichnung \\ \hline
 $\mathbf{0}$                   & Matrix oder Vektor mit Null-Elementen\\
 $\mathbf{1}$                   & Matrix oder Vektor mit Eins-Elementen\\
 2CV                            & zweifache Crossvalidierung \\
 2D                             & zweidimensional \\
 3D                             & dreidimensional \\
 5CV                            & f\"{u}nffache Crossvalidierung \\
 $a, a_i$                       & Parameter (allgemein) \\
 $\mathbf{a}$                   & 1. Transformationsvektor auf ein transformiertes Merkmal in der linearen Merkmalstransformation,
                                  2. Parametervektor (allgemein)\\
 $\mathbf{A}$                   & Transformationsmatrix in der linearen Merkmalstransformation \\
 $\mathbf{\tilde{a}}$           & Eigenvektor \\
 $\mathbf{\tilde{A}}$           & Transformationsmatrix aus Eigenvektoren \\
 $A(z)$                         & Parameterpolynom in einer $z$-\"{U}bertragungsfunktion \\
 $a_0$                          & Absolutwert\\
 $A1-3$                         & Neuronen in Ausgabeschicht \\
 $\mathbf{A}_{Faktor}$          & Transformationsmatrix in der Faktoranalyse \\
 $\mathbf{a}_H$                 & Transformationsvektor auf ein transformiertes Merkmal in einem h\"{o}herdimensionalen Raum bei SVMs\\
 $\mathbf{a}_l$                 & Vektor der Parameter der Zugeh\"{o}rigkeitsfunktionen aller Terme des Merkmals $x_l$\\
 \hline
 \end{tabular}

 \noindent
 \begin{tabular}{|p{.15\textwidth}||p{.79\textwidth}|}
 \hline
 Symbol&Bezeichnung \\ \hline
 $a_{l,i}$                      & Parameter der Zugeh\"{o}rigkeitsfunktion des Terms $A_{l,i}$ ($i=1$: rechtes Maximum
                                  Trapez-ZGF, $i=m_l$: linkes   Maximum Trapez-ZGF, $i=2,\ldots,m_l-1$: Maximum Dreieck-ZGF) \\
 $A_{l,i}$                      & $i$-ter linguistischer Term des $l$-ten Merkmals $x_l$ \\
 $a_{l,i}^{Start}$              & Startiteration f\"{u}r Parameter der Zugeh\"{o}rigkeitsfunktion des Terms $A_{l,i}$ \\
 $A_{l,R_r}$                    & ODER-Verkn\"{u}pfung linguistischer Terme des $l$-ten Merkmals $x_l$ in der Teilpr\"{a}misse der $r$-ten Regel\\
 $A_z$                          & AUC-Wert \\
 AK                             & Bewertung mit A-priori-Wahrscheinlichkeiten und Kosten \\
 ALS                            & Amyotrophe Lateralsklerose \\
 ANFIS                          & Adaptive Network based Fuzzy Inference System \\
 ANOVA                          & (univariate) Varianzanalyse (ANalysis Of VAriances)\\
 AR                             & Autoregressives Modell (siehe Tabelle~\ref{tab:armax} auf S.~\pageref{tab:armax})\\
 AR1-3                          & Koeffizienten eines autoregressiven Modells \\
 $\operatorname{argmax}$        & Argument mit dem maximalen Wert \\
 $\operatorname{argmin}$        & Argument mit dem minimalen Wert \\
 ARIMA                          & AutoRegressive Integrated Moving Average model \\
 ARIMAX                         & AutoRegressive Integrated Moving Average model with eXternal input \\
 ARMA                           & AutoRegressive Moving Average model (siehe Tabelle~\ref{tab:armax} auf S.~\pageref{tab:armax})\\
 ARMAX                          & AutoRegressive Moving Average model with eXternal input \newline (siehe Tabelle~\ref{tab:armax} auf S.~\pageref{tab:armax})\\
 ASIA                           & American Spinal Cord Injury Association \\
 AUC                            & Fl\"{a}che unter der ROC-Kurve (Area under Curve) \\
 AW                             & Bewertung mit A-priori-Wahrscheinlichkeiten und wahrscheinlichster Entscheidung \\
 $b, b_i$                       & Parameter \\
 $\mathbf{B}$                   & Zwischenklassenvariationsmatrix der Merkmale~-- Dimension $(s,s)$\\
 $B(z)$                         & Parameterpolynom einer $z$-\"{U}bertragungsfunktion \\
 $b_c$                          & 1. Parameter (allgemein),\newline
                                  2. Parameter der Zugeh\"{o}rigkeitsfunktion des Terms $B_c$  \\
 $B_c$                          & $c$-ter linguistischer Term der Ausgangsgr\"{o}{\ss}e y \\
 $B_{Rausch}$                   & Rauschcluster \\
 BCI                            & Brain Computer Interface \\
 BJ                             & Box-Jenkins model (siehe Tabelle~\ref{tab:armax} auf S.~\pageref{tab:armax})\\
 BMI                            & Brain Machine Interface \\
 BP                             & Bandpower (spektrale Leistungsdichte) \\
 BP10                           & Bandpower 10-12~Hz (spektrale Leistungsdichte) \\
 BP16                           & Bandpower 16-24~Hz (spektrale Leistungsdichte) \\
 $c$                            & Laufindex f\"{u}r Klassen \\
 $C$                            & 1. Anzahl Cluster, \newline 2. Wichtungsfaktor zur Bestrafung von Klassifikationsfehlern bei SVMs \\
 $C(z)$                         & Parameterpolynom einer $z$-\"{U}bertragungsfunktion \\
 $c_i$                          & Parameter von $C(z)$\\
 $C_r$                          & 1. Konklusion der $r$-ten Regel, 2. $r$-ter Klassifikator \\
 C3                             & EEG-Sensor (Lage siehe Bild~\ref{fig:eeg2010}) \\
 C4                             & EEG-Sensor (Lage siehe Bild~\ref{fig:eeg2010}) \\
 C4.5                           & spezieller Algorithmus f\"{u}r Entscheidungsb\"{a}ume \\
\hline
 \end{tabular}

 \noindent
 \begin{tabular}{|p{.15\textwidth}||p{.79\textwidth}|}
 \hline
 Symbol&Bezeichnung \\ \hline
 CAD                            & Computer Aided Detection  \\
 $\operatorname{card} $         & Kardinalit\"{a}t (Anzahl von Elementen einer Menge) \\
 CART                           & Classification and Regression Tree \\
 CCD                            & Charge Coupled Device (elektronisches Bauelement, das u.\,a. bei Kameras verwendet wird)\\
 COG                            & Schwerpunktmethode (Center of Gravity) \\
 COGS                           & Schwerpunktmethode f\"{u}r Singletons (Center of Gravity for Singletons) \\
 CT                             & Computertomographie\\
 CV                             & Crossvalidierung \\
 Cz                             & EEG-Sensor (Lage siehe Bild~\ref{fig:eeg2010})\\
 $d$                            & Distanz \\
 $D(z)$                         & Parameterpolynom einer $z$-\"{U}bertragungsfunktion \\
 $d_{Bat}$                      & \"{A}hnlichkeitsma{\ss} nach Bhattacharyya \\
 $d_c$                          & 1. Distanz zur $c$-ten Klasse der Ausgangsgr\"{o}{\ss}e, \newline
                                  2. Parameter in einer $z$-\"{U}bertragungsfunktion \\
 $d_{Euk}$                      & Euklidische Distanz \\
 $D_i$                          & Aufgaben und Bewertungsma{\ss}e im Data Mining (Entwurf), \newline siehe Tabellen~\ref{tab:problemklassen_prog},~\ref{tab:problemklassen_merk} und~\ref{tab:problemklassen_bewert} \\
 $D_{iA}$                       & Aufgaben und Bewertungsma{\ss}e im Data Mining (Anwendung), \newline  siehe Tabellen~\ref{tab:problemklassen_anwendung},~\ref{tab:problemklassen_anwendung_merk}   \\
 $d_{KL}$                       & Divergenz nach Kullback-Leibler \\
 $d_{KL,min}$                   & untere Absch\"{a}tzung der Divergenz nach Kullback-Leibler \\
 $d_{Mah}$                      & Mahalanobis-Distanz \\
 $d_{Man}$                      & Manhattan-Distanz \\
 $d_{Mink}$                     & Minkowski-Distanz \\
 $d_{QF,\mathbf{W}_{QF}}$       & Distanz mit quadratischer Form \\
 $d_{Rausch}$                   & Konstante, die Distanz zum Rauschcluster angibt \\
 $d_{Tr}$                       & Triviale Distanz \\
 DA                             & Diskriminanzanalyse \\
 $\operatorname{det}$           & Determinante einer Matrix\\
 $\operatorname{diag}$          & Diagonalmatrix \\
 DNA                            & Desoxyribonukleins\"{a}ure \\
 DS                             & Datensatz \\
 DSP                            & Digitaler Signalprozessor \\
 DSS                            & Entscheidungsunterst\"{u}tzendes System (Decision Support System) \\
 $E(\cdot)$                     & Erwartungswert \\
 E1-E3                          & Neuronen in Eingangsschicht \\
 $E_i$                          & Ereignis (allgemein) \\
 EBM                            & Evidenz-basierte Medizin \\
 ECoG                           & Elektrokortikographie \\
 EEG                            & Elektroencephalogramm \\
 EK                             & Entscheidungskosten \\
 EKG                            & Elektrokardiogramm \\
 EMG                            & Elektromyogramm\\
 ENG                            & Elektroneurogramm \\
 ERD                            & Event-related Desynchronization \\
 \hline
 \end{tabular}

 \noindent
 \begin{tabular}{|p{.15\textwidth}||p{.79\textwidth}|}
 \hline
 Symbol&Bezeichnung \\ \hline
 ERS                            & Event-related Synchronization \\
 ESS                            & erkl\"{a}rte Streuung (Explained Sum of Squares) \\
 EU                             & Euklidische Distanz \\
 $\exp$                         & Exponentialfunktion \\
 $\mathbf{F}$                   & Matrix mit transformierten Merkmalen bei Regressionsproblemen, \newline  Dimension $(N,s_f)$\\
 $f(\cdot)$                     & allgemeine Funktion \\
 $F(z)$                         & Parameterpolynom einer $z$-\"{U}bertragungsfunktion \\
 $f_i$                          & Parameter \\
 $F_p(x)$                       & Verteilungsfunktion \\
 $f_r(\cdot)$                   & $r$-te Funktion \\
 $F_r$                          & Anzahl fehlerhaft klassifizierter Datentupel der $r$-ten Regel \\
 $f_{TP}(\cdot)$                & Hilfsfunktion bei der Implementierung von Fuzzy-Systemen\\
 FCM                            & Fuzzy-C-Means \\
 FDA                            & Food and Drug Association \\
 FFT                            & Fast Fourier Transformation \\
 FIR                            & Finite Input Response \\
 fMRT                           & funktionelle Magnetresonanztomographie \\
 FN                             & False Negative (Anzahl der falsch klassifizierten Datentupel  mit $y=B_c$ und Entscheidung $\hat{y}=\overline{B}_c$)  \\
 FP                             & False Positive (Anzahl der falsch klassifizierten Datentupel mit $y=\overline{B}_c$ und Entscheidung $\hat{y}=B_c$)  \\
 fro                            & frontale Ebene (von vorn) \\
 $g(\cdot)$                     & allgemeine Funktion \\
 GK                             & Gustafson-Kessel-Algorithmus \\
 GZR                            & Geschwindigkeitszeitreihe \\
 $\mathbf{H}$                   & Hesse-Matrix \\
 $H(\cdot)$                     & 1. Entropie, \newline 2. kumuliertes Sterberisiko bei der Sch\"{a}tzung von \"{U}berlebenszeiten\\
 $h(t)$                         & Sterberisiko (Hasard) \\
 $H(x)$                         & Eingangsentropie\\
 $H(x,y)$                       & Gesamtentropie der Gr\"{o}{\ss}en $x, y$ \\
 $H(x;y)$                       & Transinformation \\
 $H(x|y)$                       & \"{A}quivokation (R\"{u}ckschlussentropie) \\
 $H(y)$                         & Ausgangsentropie\\
 $H(y|x)$                       & Irrelevanz \\
 $H_0$                          & Nullhypothese bei statistischen Tests\\
 $h_0(t)$                       & Referenzkurve f\"{u}r das Sterberisiko (Hasard) \\
 $H_1$                          & Alternativhypothese bei statistischen Tests (Gegenteil der Nullhypothese)\\
 $H_i(\cdot)$                   & Entropie in einem Teil des Datensatzes \newline (z.\,B.  in einem Knoten eines Entscheidungsbaums) \\
 HK                             & Hauptkomponentenanalyse ohne Varianznormierung\\
 HKA                            & Hauptkomponentenanalyse (allgemein) \\
 HKS                            & Hauptkomponentenanalyse mit Varianznormierung\\
 $i$                            & Laufindex \\
 $\mathbf{I}$                   & Einheitsmatrix \\
 \hline
 \end{tabular}

 \noindent
 \begin{tabular}{|p{.15\textwidth}||p{.79\textwidth}|}
 \hline
 Symbol&Bezeichnung \\ \hline
 $\mathbb{I}$                  & Indexmenge f\"{u}r Merkmale \\
 $i_G$                          & Nummer des Gewinnerneurons  \\
 $\mathbb{I}_k$                & Indexmenge f\"{u}r Kategorien \\
 $\mathbb{I}_{k-NN}$           & Indexmenge mit den $k$ n\"{a}chsten Nachbarn \\
 $i_x$                          & Laufindex f\"{u}r Spalten in einem Bild \\
 $I_x$                          & Anzahl Spalten in einem Bild \\
 $i_y$                          & Laufindex f\"{u}r Zeilen in einem Bild \\
 $I_y$                          & Anzahl Zeilen in einem Bild \\
 $i_z$                          & Laufindex f\"{u}r Schichten in einem dreidimensionalen Bild \\
 $I_z$                          & Anzahl Schichten in einem dreidimensionalen Bild \\
 ICA                            & Unabh\"{a}ngigkeitsanalyse (Independent Component Analysis) \\
 ICP                            & Infantile Zerebralparese \\
 ID                             & Identifikationsnummer \\
 ID3                            & spezieller Algorithmus f\"{u}r Entscheidungsb\"{a}ume \\
 IIR                            & Infinite Input Response \\
 ISw                            & Initial Swing (5. Schrittphase) \\
 $j$                            & Laufindex \\
 $k$                            & 1. Abtastzeitpunkt (in eckigen Klammern), \newline
                                  2. Anzahl Nachbarn bei $k$-Nearest-Neighbor-Klassifikatoren \\
 $K$                            & Anzahl Abtastzeitpunkte \\
 $K(\cdot,\cdot)$               & Kernoperation \\
 $K_{neg}$                      & Faktor bei der Berechnung von Konfidenzintervallen f\"{u}r Regeln \\
 $K_{pos}$                      & Faktor bei der Berechnung von Konfidenzintervallen f\"{u}r Regeln \\
 $K_{stat}$                     & Sicherheitsfaktor f\"{u}r Fehlerabsch\"{a}tzungen der Entropie \\
 $k_{Tot} $                     & diskrete Totzeit \\
 $\mathbf{K}_x$                 & Matrix der Merkmalskategorien \\
 KDD                            & Knowledge Discovery in Databases \\
 $k$-NN                         & $k$-Nearest Neighbor \\
 KNN                            & K\"{u}nstliches Neuronales Netz \\
 KO                             & Knock Out \\
 $l$                            & Laufindex \\
 $L$                            & 1. Kosten (allgemein), 2. linke K\"{o}rperseite (Bewegungsanalyse) \\
 $L(\hat{y}=B_c |$\newline \phantom{$L($}$y=B_i)$   & Kosten f\"{u}r eine (Fehl-) Entscheidung zu Gunsten von Klasse $B_c$ f\"{u}r ein Datentupel der Klasse $B_i$ \\
 $L_{fix,l}$                    & fixe Kosten f\"{u}r die Berechnung eines Merkmals $x_l$ \\
 $l_k$                          & Laufindex f\"{u}r Kategorien \\
 $L_{var,l}$                    & variable Kosten f\"{u}r die Berechnung eines Datentupels des Merkmals $x_l$ \\
 LD                             & Lerndatensatz \\
 LM                             & Linkes Maximum \\
 $\ln$                          & nat\"{u}rlicher Logarithmus \\
 $\log_2$                       & Logarithmus zur Basis 2\\
 $\operatorname{logit}$         & Logit-Funktion\\
 LOLIMOT                        & Local linear model trees  \\
 LR                             & Loading Response (1. Schrittphase) \\
 LS                             & Least Square \\
 LVQ                            & Lernende Vektorquantisierung \\
 \hline
 \end{tabular}

 \noindent
 \begin{tabular}{|p{.15\textwidth}||p{.79\textwidth}|}
 \hline
 Symbol&Bezeichnung \\ \hline
 $m$                            & 1. Parameter (Mittelwert), \newline
                                  2. Anzahl der linguistischen  Terme aller Merkmale \\
 $\mathbf{M}_i$                 & Matrix (allgemein) \\
 $m_l$                          & Anzahl der linguistischen Terme des $l$-ten Merkmals $x_l$ \\
 $m_y$                          & Anzahl der linguistischen Terme (Klassen) der Ausgangsgr\"{o}{\ss}e  \\
 MA                             & Moving Average model (siehe Tabelle~\ref{tab:armax} auf S.~\pageref{tab:armax})\\
 MAN, \newline MANOVA           & multivariate Varianzanalyse (Multivariate ANalysis Of VAriances)\\
 MAPO                           & Maximumposition: zugeh\"{o}riger Abtastzeitpunkt zum Maximum \\
 $\max$, MAX                    & Maximum \\
 MD                             & Modifizierte Diskriminanzanalyse \\
 MDL                            & Minimum Description Length\\
 MEG                            & Magnetoencephalographie \\
 MIMO                           & System mit mehreren Ein- und Ausg\"{a}ngen \newline (Multiple Input Multiple Output)\\
 $\min$, MIN                    & Minimum \\
 MIPO                           & Minimumposition: zugeh\"{o}riger Abtastzeitpunkt zum Minimum \\
 MISO                           & System mit mehreren Eing\"{a}ngen und einem Ausgang \newline (Multiple Input Single Output)\\
 MKQ                            & Methode der kleinsten Fehler-Quadrate \\
 MLP                            & Multi-Layer Perceptron \\
 MM                             & Modifizierte Merkmalsselektion \\
 MML                            & Minimum Message Length\\
 MOM                            & Mean of Maximum \\
 MRI                            & Magnetresonanztomographie (Magnetic Resonance Imaging) \\
 MRT                            & Magnetresonanztomographie \\
 MSt                            & Mid Stance (2. Schrittphase) \\
 MSw                            & Mid Swing (6. Schrittphase) \\
 MW                             & Mittelwert \\
 $n$                            & 1. Laufindex Datentupel, 2. allgemeine Bezeichnung f\"{u}r eine Anzahl\\
 $N$                            & Anzahl Datentupel \\
 $\mathbb{N}$                   & Menge der nat\"{u}rlichen Zahlen \\
 $N(x_l=A_{l,i})$               & Anzahl des Auftretens der Klasse $A_{l,i}$ f\"{u}r das Merkmal $x_l$\\
 $N(x_l= A_{l,i}\cap$\newline \phantom{$N/$}$y= B_c)$   & Anzahl des Auftretens der UND-Verkn\"{u}pfung von $x_l=A_{l,i}$ und $y=B_c$ \\
 $N(y=B_c)$                     & Anzahl des Auftretens der Ausgangsklasse $B_c$\\
 $N300$                         & negativer Peak in einem EEG-Signal 300~ms nach einem Ereignis \\
 $n_a$                          & Ordnung eines Polynoms $A(z)$ \\
 $N_{Anw}$                      & Anzahl auszuwertender Datentupel in der Anwendungsphase \\
 $n_b$                          & Ordnung eines Polynoms $B(z)$ \\
 $n_c$                          & Ordnung eines Polynoms $C(z)$ \\
 $N_c$                          & Anzahl Datentupel der $c$-ten Ausgangsklasse \\
 $n_{Cl}$                       & Laufindex Klassifikatoren bei Klassifikatorfusion \\
 $N_{Cl}$                       & Anzahl Klassifikatoren bei Klassifikatorfusion \\
 $n_d$                          & Ordnung eines Polynoms $D(z)$ \\
 $N_{\text{Diagnose c}}$        & Anzahl Patienten mit einer Diagnose $c$\\
 $n_{EB}$                       & Anzahl generierter Entscheidungsb\"{a}ume \\
 \hline
 \end{tabular}

 \noindent
 \begin{tabular}{|p{.15\textwidth}||p{.79\textwidth}|}
 \hline
 Symbol&Bezeichnung \\ \hline
 $n_f$                          & Ordnung eines Polynoms $F(z)$ \\
 $N_F$                          & Anzahl an Freiheitsgraden einer Verteilung \\
 $N_{Hyp}$                      & Anzahl getesteter Hypothesen \\
 $N_i$                          & Anzahl Datentupel im  Knoten $v_i$ eines Entscheidungsbaums \\
 $N_{Knoten}$                   & Anzahl Knoten in einem Entscheidungsbaum\\
 $N_{Lern}$                     & Anzahl Datentupel im Lerndatensatz\\
 $N_{mod}$                      & Anzahl ausgew\"{a}hlter Datentupel nach einer Datentupelselektion\\
 $N_{\text{Population}}$        & Anzahl Personen in einem untersuchten Kollektiv\\
 $N_r$                          & Anzahl abgedeckter Datentupel durch die Pr\"{a}misse der $r$-ten Regel \\
 $N_S[k]$                       & Anzahl der zum Zeitpunkt $k$ lebenden Personen \\
 $N_{Schritt,Pat_i}             $& Anzahl aller aufgenommenen Schritte des $i$-ten Patienten \\
 $N_T[k]$                       & Anzahl der im Zeitraum zwischen $k-1$ und $k$ verstorbenen Personen \\
 $N_{Test}$                     & Anzahl Datentupel im Testdatensatz\\
 $n_x$                          & Anzahl einbezogener vergangener Abtastzeitpunkte f\"{u}r die Merkmale \\
 $n_y$                          & Anzahl einbezogener vergangener Abtastzeitpunkte f\"{u}r die Ausgangsgr\"{o}{\ss}e \\
 NARMAX                         & Nonlinear AutoRegressive Moving Average model with eXternal input \\
 NEFCLASS                       & Neuro Fuzzy Approach for the Classification of Data \\
 NEG                            & linguistischer Term Negativ\\
 NG                             & linguistischer Term Negativ Gro{\ss}\\
 NK                             & linguistischer Term Negativ Klein\\
 NM                             & linguistischer Term Negativ Mittel\\
 NSG                            & linguistischer Term Negativ Sehr Gro{\ss}\\
 NSK                            & linguistischer Term Negativ Sehr Klein\\
 $O_i,O_j,O_K$                  & Objekte, Elemente einer Menge \\
 OE                             & Output error model (siehe Tabelle~\ref{tab:armax} auf S.~\pageref{tab:armax})\\
 OR                             & Odds ratio \\
 OSG                            & Oberes Sprunggelenk \\
 $p$                            & 1. Parameter, 2. Irrtumswahrscheinlichkeit bei einem statistischen Test\\
 $p(\cdot)$                     & Verteilungsdichtefunktion\\
 $P(\cdot)$                     & Wahrscheinlichkeit\\
 $\mathbf{\hat{P}}$             & Vektor oder Matrix der Wahrscheinlichkeiten f\"{u}r Klassen einer skalaren Ausgangsgr\"{o}{\ss}e \\
 P$+$                           & F\"{o}rderrichtung Pumpe in Richtung Aktor \\
 P$-$                           & F\"{o}rderrichtung Pumpe aus Aktor heraus\\
 P$\pm$                         & F\"{o}rderrichtung Pumpe in Richtung Aktor bzw. aus Aktor heraus\\
 $p(\mathbf{x}|y=B_c)$          & bedingte Wahrscheinlichkeit von $\mathbf{x}$ f\"{u}r die Ausgangsklasse $y=B_c$ \newline ($\mathbf{x}$ mehrdimensional und reell) \\
 $P(x_l=A_{l,i})$               & Wahrscheinlichkeit des Auftretens der Klasse $A_{l,i}$ f\"{u}r das Merkmal $x_l$\\
 $P(x_l= A_{l,i}\cap$\newline \phantom{$P/$}$y= B_c)$   & Wahrscheinlichkeit der UND-Verkn\"{u}pfung von $x_l=A_{l,i}$ und $y=B_c$ \\
 $P(y=B_c)$                     & Wahrscheinlichkeit der Ausgangsklasse $y=B_c$ \\
 $P(y=B_c|\mathbf{x})$          & bedingte Wahrscheinlichkeit der Ausgangsklasse $y=B_c$ f\"{u}r $\mathbf{x}$ \newline ($\mathbf{x}$ mehrdimensional und reell)\\
 $\mathbf{\hat{P}}(y|x_l)$      & Matrix der gesch\"{a}tzten bedingten Wahrscheinlichkeiten
                                  f\"{u}r die Ausgangsklassen von $y$ f\"{u}r die $m_l$ Klassen des Merkmals $x_l$ f\"{u}r einen Datensatz\\
 \hline
 \end{tabular}

 \noindent
 \begin{tabular}{|p{.15\textwidth}||p{.79\textwidth}|}
 \hline
 Symbol&Bezeichnung \\ \hline
 $p_c(\cdot)$                   & Verteilungsdichtefunktion der Merkmale f\"{u}r die Ausgangsklasse $y=B_c$ \\
 $\mathbf{p}_i$                 & $i$-ter Positionsvektor bei Kohonen-Karten\\
 $P_{ob}(\cdot)$                & obere Schranke einer Wahrscheinlichkeit\\
 $P_{un}(\cdot)$                & untere Schranke einer Wahrscheinlichkeit\\
 P300                           & positiver Peak in einem EEG-Signal 300~ms nach einem Ereignis\\
 PAT                            & Patientenkollektiv \\
 $PAT_i$                        & $i$-ter Patient\\
 PC                             & Personalcomputer \\
 PCA                            & Hauptkomponentenanalyse (Principal Component Analysis) \\
 PET                            & Positronenemissionstomographie \\
 PG                             & linguistischer Term Positiv Gro{\ss}\\
 PK                             & linguistischer Term Positiv Klein\\
 PM                             & linguistischer Term Positiv Mittel\\
 POS                            & linguistischer Term Positiv\\
 POST                           & posttherapeutisches Patientenkollektiv \\
 PRE                            & pr\"{a}therapeutisches Patientenkollektiv \\
 PROB                           & Probandenkollektiv \\
 PSG                            & linguistischer Term Positiv Sehr Gro{\ss}\\
 PSK                            & linguistischer Term Positiv Sehr Klein\\
 PSw                            & Pre Swing (4. Schrittphase) \\
 $q$                            & Fuzzifier bei Clusterverfahren \\
 $Q$                            & Bewertungsma{\ss} (allgemein) \\
 $Q_{Cluster}$                  & Bewertungsma{\ss} beim (scharfen) Clustering \\
 $Q_D$                          & Entscheidungskosten \\
 $Q_{D,r}$                      & Entscheidungskosten f\"{u}r die $r$-te Regel\\
 $Q_{D,r_{opt}}$                & geringste Entscheidungskosten einer Regel aus mehreren Alternativen\\
 $Q_F$                          & Kosten zur Auswertung eines Modells $f(\cdot)$  \\
 $Q_{F0}$                       & Kosten zur Auswertung eines Modells $f(\cdot)$ ohne Merkmalskosten \\
 $Q_{F,l}$                      & Kosten zur Berechnung des Merkmals $x_l$ \\
 $Q_{F,r}$                      & Kosten zur Auswertung eines Modells $f(\cdot)$ f\"{u}r die $r$-te Regel \\
 $Q_{Fuzzy-Cluster}$            & Bewertungsma{\ss} Fuzzy-Clustering \\
 $Q_{Gini}$                     & Gini-Index\\
 $Q_K$                          & Klassifikationsfehler \\
 $Q_{K,0}$                      & Klassifikationsfehler eines Trivialmodells \\
 $Q_{K,G}$                      & Klassifikationsg\"{u}te \\
 $Q_{K,GV}$                     & Verbesserung der Klassifikationsg\"{u}te im Vergleich zu einem Trivialmodell\\
 $Q_{Klar}$                     & Klarheit \\
 $Q_{Klar,r}$                   & Klarheit einer Regel\\
 $Q_{Kp}$                       & Klassifikationsfehler \"{u}ber gesch\"{a}tzte Wahrscheinlichkeiten von\newline Fehlklassifikationen \\
 $Q_{Kp,0}$                     & Klassifikationsfehler \"{u}ber gesch\"{a}tzte Wahrscheinlichkeiten von\newline Fehlklassifikationen eines Trivialmodells\\
 $Q_{Kp,G}$                     & Klassifikationsg\"{u}te \"{u}ber gesch\"{a}tzte Wahrscheinlichkeiten von \newline Fehlklassifikationen \\
 $Q_{Kp,GV}$                    & Verbesserung der Klassifikationsg\"{u}te \"{u}ber gesch\"{a}tzte Wahrscheinlichkeiten von Fehlklassifikationen im Vergleich zu einem Trivialmodell\\
 \hline
 \end{tabular}

 \noindent
 \begin{tabular}{|p{.15\textwidth}||p{.79\textwidth}|}
 \hline
 Symbol&Bezeichnung \\ \hline
 $Q_{Kw}$                       & gewichteter Klassifikationsfehler \\
 $Q_l$                          & Merkmalsbewertung (allgemein) \\
 $Q_L$                          & Bewertungsma{\ss} in Lagrange-Formulierung bei SVMs \\
 $Q_{Lern}$                     & beliebiges Bewertungsma{\ss} f\"{u}r den Lerndatensatz \\
 $Q_{NR}$                       & nichtrestringiertes Bewertungsma{\ss} bei SVMs \\
 $Q_{PD}$                       & Pr\"{a}ferenz einer Entscheidung \\
 $Q_{PF}$                       & Pr\"{a}ferenz zur Auswertung eines Modells $f(\cdot)$  \\
 $Q_{PF,0}$                     & Pr\"{a}ferenz zur Auswertung eines Modells $f(\cdot)$ ohne Pr\"{a}ferenzen\newline von Merkmalen \\
 $Q_{PF,Imp}$                   & Pr\"{a}ferenz bez\"{u}glich der Implementierbarkeit \\
 $Q_{PF,Int}$                   & Pr\"{a}ferenz bez\"{u}glich der Interpretierbarkeit \\
 $Q_{PF,l}$                     & Merkmalspr\"{a}ferenz $x_l$ \\
 $Q_{PFK,l_k}$                  & Pr\"{a}ferenz der $l_k$-ten Merkmalskategorie  \\
 $Q_{PT}$                       & Gesamtpr\"{a}ferenz (Entscheidung und Modell) \\
 $Q_{R^2,F}$                    & Bestimmtheitsma{\ss} mit Frobenius-Norm \\
 $Q_{R^2,Norm}$                 & Bestimmtheitsma{\ss} mit einer beliebigen Norm \\
 $Q_{red}(\cdot,\cdot)$         & Redundanzma{\ss} \\
 $Q_{RS}$                       & Bewertungsma{\ss} nach einer R\"{u}ckstufung redundanter Merkmale \\
 $Q_{Sens,c}$                   & Sensitivit\"{a}t f\"{u}r Klasse $B_c$ (ohne $c$: f\"{u}r nur eine Klasse und ihre Negation) \\
 $Q_{Spez,c}$                   & Spezifit\"{a}t f\"{u}r Klasse $B_c$ (ohne $c$: f\"{u}r nur eine Klasse und ihre Negation) \\
 $Q_{Stat}$                     & statistische Absicherungsg\"{u}te \\
 $Q_T$                          & Gesamtkosten (Entscheidungs- und Modellkosten) \\
 $Q_{Test}$                     & beliebiges Bewertungsma{\ss} f\"{u}r den Testdatensatz \\
 $Q_{Trenn}$                    & Trennungsgrad \\
 $Q_{Twoing}$                   & Twoing-Index \\
 $r$                            & Laufindex Regel\\
 $R$                            & rechte K\"{o}rperseite (Bewegungsanalyse)\\
 $\mathbb{R}$                   & Menge der reellen Zahlen \\
 $R^2$                          & Bestimmtheitsma{\ss} \\
 $r_e$                          & letzter linguistischer Term in der ODER-Verkn\"{u}pfung einer Teilpr\"{a}misse\\
 $r_{max}$                      & Anzahl Regeln in Regelbasis\\
 $R_r$                          & $r$-te Regel \\
 $r_s$                          & erster linguistischer Term in der ODER-Verkn\"{u}pfung einer Teilpr\"{a}misse\\
 $R_s$                          & Spearman-Korrelationskoeffizient \\
 $r_{sonst}$                    & Nummer der Sonst-Regel\\
 $R_{SpW,l}$                    & Spannweite eines Merkmals $x_l$ \\
 $r_{y,\hat{y}}$                & empirischer Korrelationskoeffizient zwischen  $y$ und $\hat{y}$\\
 RB                             & Regelbasis \\
 RCT                            & Randomized Controlled Trials \\
 $\operatorname{rd}$            & Rundungsoperator \\
 RM                             & Rechtes Maximum \\
 ROC                            & Receiver Operator Characteristic \\
 ROSA                           & Regelorientierte Statistische Analyse\\
 RRG                            & Relative Regressionsg\"{u}te \\
 RSS                            & nicht erkl\"{a}rte Streuung (Residual Sum of Squares) \\
 \hline
 \end{tabular}

 \noindent
 \begin{tabular}{|p{.15\textwidth}||p{.79\textwidth}|}
 \hline
 Symbol&Bezeichnung \\ \hline
 RU                             & Runden \\
 RZR                            & Referenzabweichungszeitreihe \\
 $s$                            & Anzahl der Merkmale \\
 $\mathbf{S}$                   & Sch\"{a}tzung der Kovarianzmatrix der Merkmale\\
 $S(t)$                         & erwartete \"{U}berlebensrate \\
 $s_b$                          & Anzahl der Bilder, die zu einem Datentupel geh\"{o}ren\\
 $\mathbf{S}_c$                 & Sch\"{a}tzung der Kovarianzmatrix der Merkmale f\"{u}r die $c$-te Ausgangsklasse\\
 $\mathbf{S}_{c,Reg}$           & wie $\mathbf{S}_c$, aber mit zus\"{a}tzlicher Regularisierung  \\
 $s_d$                          & Anzahl der transformierten Merkmale \\
 $s_{dx}$                       & Anzahl einbezogener Rohmerkmale (Abtastzeitpunkte und Merkmale) bei der Merkmalsextraktion f\"{u}r dynamische Systeme\\
 $s_{dy}$                       & Anzahl einbezogener Rohmerkmale (Abtastzeitpunkte und Ausgangsgr\"{o}{\ss}en) bei der Merkmalsextraktion f\"{u}r dynamische Systeme\\
 $s_{Ebene}$                    & Anzahl Neuronen in einer Ebene einer Kohonen-Karte \\
 $s_f$                          & Anzahl der Merkmale bei Regressionsans\"{a}tzen\\
 $\mathbf{S}_{F,c}$             & Fuzzy-Kovarianzmatrix \\
 $S_G$                          & Nummer Generalisierungsschritt beim Generalisieren von Einzelregeln \\
 $s_k$                          & Anzahl der Kategorien \\
 $s_{KNN}$                      & Parameteranzahl eines K\"{u}nstlichen Neuronalen Netzes \\
 $s_m$                          & Anzahl der ausgew\"{a}hlten Merkmale \\
 $s_{Neuron,i}$                 & Anzahl der Neuronen in der $i$-ten Schicht eines K\"{u}nstlichen \newline Neuronalen Netzes \\
 $s_{Roh}$                      & Anzahl der Rohmerkmale \\
 $s_{Schicht}$                  & Anzahl der Schichten eines K\"{u}nstlichen Neuronalen Netzes \\
 $s_v$                          & Anzahl der Videos, die zu einem Datentupel geh\"{o}ren\\
 $s_y$                          & Anzahl der Ausgangsgr\"{o}{\ss}en \\
 $s_z$                          & Anzahl der Zeitreihen, die zu einem Datentupel geh\"{o}ren \\
 sag                            & sagittale Ebene (seitlich) \\
 SAMS                           & Southampton Adaptive Manipulation Scheme \\
 SCP                            & Slow Cortical Potentials \\
 SICA                           & r\"{a}umliche Unabh\"{a}ngigkeitsanalyse \newline (Spatial Independent Component Analysis) \\
 SISO                           & System mit einem Ein- und einem Ausgang (Single Input Single Output)\\
 SOFM                           & Kohonen-Karte (Self Organizing Feature Map) \\
 SOM                            & Kohonen-Karte (Self Organizing Map) \\
 $\operatorname{sp}$            & Spur einer Matrix \\
 SPECT                          & Single-Photon-Emission-Computertomographie\\
 SpW                            & Spannweite \\
 SSCP                           & Gesamtstreuung (Sum of Square and Cross Products) \\
 SSE                            & nicht erkl\"{a}rte Streuung (Sum of Squares Error) \\
 St                             & Standphase (Stand phase) \\
 STD                            & Standardabweichung \\
 Stri                           & Stride (Doppelschritt) \\
 SVM                            & Support-Vektor-Maschine \\
 Sw                             & Schwungphase (Swing phase) \\
 SZR                            & Standardabweichungszeitreihe \\
 \hline
 \end{tabular}

 \noindent
 \begin{tabular}{|p{.15\textwidth}||p{.79\textwidth}|}
 \hline
 Symbol&Bezeichnung \\ \hline
 $t$                            & Zeit (wertekontinuierlich) \\
 $\mathbf{T}$                   & Gesamtvariationsmatrix der Merkmale~-- Dimension $(s,s)$\\
 $T^2$                          & Spur-Statistik \\
 $T_A$                          & Abtastzeit\\
 $t_i$                          & bestimmter Zeitpunkt\\
 $T_{\emph{name}}$              & Textrahmen f\"{u}r Erkl\"{a}rungstexte \\
 $t_{POST}$                     & Zeitpunkt einer Messung nach einer Therapie\\
 $t_{PRE}$                      & Zeitpunkt einer Messung vor einer Therapie\\
 $t_{THER}$                     & Zeitpunkt einer Therapie\\
 THER                           & Therapie\\
 TICA                           & zeitliche Unabh\"{a}ngigkeitsanalyse \newline (Temporal Independent Component Analysis) \\
 TP                             & True Positive (Anzahl richtig klassifizierter Datentupel einer Klasse $B_c$) \\
 TN                             & True Negative (Anzahl richtig klassifizierter Datentupel einer Klasse $\overline{B}_c$) \\
 tra                            & transversale Ebene (von oben) \\
 TSS                            & Gesamtstreuung (Total Sum of Squares) \\
 TSt                            & Terminal Stance (3. Schrittphase) \\
 TSw                            & Terminal Swing (7. Schrittphase) \\
 $u (t), \mathbf{u} (t)$        & skalare bzw. vektorielle Eingangsgr\"{o}{\ss}e eines dynamischen Systems \\
 $U(z)$                         & $z$-Transformierte der Eingangsgr\"{o}{\ss}e $u$ \\
 $U^\star$                      & Produktkriterium \\
 V1-6                           & 1. Ventile 1-6\newline\\
                                & 2. Neuronen in verdeckter Schicht\\
 $v_i$                          & $i$-ter Knoten eines Entscheidungsbaums \\
 $v_i (E)$                      & Endknoten eines Entscheidungsbaums \\
 $v_i (W)$                      & Wurzelknoten eines Entscheidungsbaums \\
 $V_r$                          & Pr\"{a}misse der $r$-ten Regel \\
 $V_{r,l}$                      & $l$-te Teilpr\"{a}misse der Pr\"{a}misse der $r$-ten Regel \\
 VAS                            & Visuelle Analogskala \\
 VC                             & Vapnik-Chervonensky-Dimension \\
 VDF                            & Verteilungsdichtefunktion \\
 VN                             & Varianznormierung \\
 $\mathbf{w}$                   & Parametervektor bei K\"{u}nstlichen Neuronalen Netzen (allgemein)\\
 $\mathbf{W}$                   & Innerklassenvariationsmatrix der Merkmale~-- Dimension $(s,s)$\\
 $w_0$                          & Absolutwert als Parameter bei K\"{u}nstlichen Neuronalen Netzen\\
 $\mathbf{w}_i$                 & Parametervektor bei K\"{u}nstlichen Neuronalen Netzen ($i$-tes Neuron)\\
 $\mathbf{w}_{MLP}$             & Parametervektor bei MLP-Netzen\\
 $\mathbf{W}_{QF}$              & Wichtungsmatrix einer quadratischen Form\\
 $\mathbf{W}_{QF,c}$            & Wichtungsmatrix einer quadratischen Form f\"{u}r das $c$-te Cluster\\
 $w_{QF,n}$                     & Diagonalelemente einer Wichtungsmatrix \\
 $\mathbf{W}_{rek}$             & Wichtungsmatrix bei der Aktualisierung von Parametervektoren\\
 $\mathbf{w}_{SOM,i}$           & Parametervektor des $i$-ten Neurons bei Kohonen-Karten\\
 WISCI                          & Walking Index for Spinal Cord \\
 $x$                            & Merkmal (allgemein) \\
 $\mathbf{X}$                   & Matrix der Merkmale ($N$ Zeilen, $s$ Spalten) \\
 $\overline{\mathbf{x}}$        & Mittelwert der Merkmale\\
 \hline
 \end{tabular}

 \noindent
 \begin{tabular}{|p{.15\textwidth}||p{.79\textwidth}|}
 \hline
 Symbol&Bezeichnung \\ \hline
 $x (t), \mathbf{x} (t)$        & skalare bzw. vektorielle Zustandsgr\"{o}{\ss}e eines dynamischen Systems \\
 $x_{Bild,l}$                   & Pixel bzw. Voxel eines 2D- oder 3D-Bildes (siehe Tabelle~\ref{tab:sroh})  \\
 $\mathbf{X}_c$                 & Matrix der Merkmale: nur Datentupel f\"{u}r Klasse $c$ ($N_c$ Zeilen, $s$ Spalten) \\
 $\overline{\mathbf{x}}_c$      & Mittelwert der Merkmale f\"{u}r Klasse $c$ \\
 $x_{D,l}$                      & Differenzmerkmal\\
 $x_{Dis,l}$                    & wertediskretes Merkmal $x_l$\\
 $x_{GZR,l}[k,n]$               & $k$-ter Abtastzeitpunkt der $l$-ten Geschwindigkeitszeitreihe \newline ($n$-tes Datentupel) \\
 $\mathbf{X}_\mathbb{I}$       & Matrix der selektierten Merkmale ($N$ Zeilen, $s_m$ Spalten) \\
 $x_l$                          & $l$-tes Merkmal\\
 $x_l[n]$                       & $n$-tes Datentupel f\"{u}r das $l$-te Merkmal im Datensatz \\
 $x_{l,krit}$                   & kritischer Wert f\"{u}r das $l$-te Merkmal (Konstante)\\
 $\bar{x}_{l,Ref}[k]$           & $k$-ter Abtastzeitpunkt des Mittelwertes der $l$-ten Zeitreihe f\"{u}r ein \newline Referenzkollektiv \\
 $x_l^{sort}[n]$                & aufsteigend sortierte Werte f\"{u}r das Merkmal $x_l$ in einem Datensatz \\
 $\mathbf{X}_{Roh}$             & Matrix der Rohmerkmale ($N$ Zeilen, $s_{Roh}$ Spalten) \\
 $x_{RZR,l}[k,n]$               & $k$-ter Abtastzeitpunkt der $l$-ten Referenzabweichungszeitreihe \newline ($n$-tes Datentupel) \\
 $x_{SZR,l,Pat_i}[k]$           & $k$-ter Abtastzeitpunkt der $l$-ten Standardabweichungszeitreihe des $i$-ten Patienten ($n$-tes Datentupel) \\
 $\mathbf{x}_{Ther}$             & Vektor der Therapieentscheidungen \\
 $x_{Trans}$                    & skalares transformiertes Merkmal \\
 $\mathbf{x}_{Trans}$           & Vektor der transformierten Merkmale ($s_d$ Spalten) \\
 $\mathbf{X}_{Trans}$           & Matrix der transformierten Merkmale ($N$ Zeilen, $s_d$ Spalten) \\
 $\mathbf{x}_{Trans,H}$         & Vektor der transformierten Merkmale in einem h\"{o}herdimensionalen \newline Merkmalsraum\\
 $x_{Video,l}$                  & Pixel bzw. Voxel eines 2D- oder 3D-Videobildes (siehe Tabelle~\ref{tab:sroh})  \\
 $ \mathbf{X}_{VN}$             & Vektor varianznormierter Merkmale \\
 $x_{ZR,l}[k,n] $               & $k$-ter Abtastzeitpunkt der $l$-ten Zeitreihe ($n$-tes Datentupel) \\
 $y$                            & skalare Ausgangsgr\"{o}{\ss}e  \\
 $\mathbf{y}$                   & Vektor der skalaren Ausgangsgr\"{o}{\ss}e ($N$ Zeilen) \\
 $\mathbf{Y}$                   & Matrix der Ausgangsgr\"{o}{\ss}e ($N$ Zeilen, $s_y$ Spalten) \\
 $y(t),\mathbf{y}(t)$           & skalare bzw. vektorielle Ausgangsgr\"{o}{\ss}e eines dynamischen Systems \\
 $Y(z)$                         & $z$-Transformierte der Ausgangsgr\"{o}{\ss}e $y$ \\
 $y_j$                          & $j$-te Ausgangsgr\"{o}{\ss}e  \\
 $y_j[n]$                       & $n$-tes Datentupel f\"{u}r die $j$-te Ausgangsgr\"{o}{\ss}e im Datensatz \\
 $y_{PatID}[n]$                 & zugeh\"{o}rige Patienten-ID des $n$-ten Datentupels \\
 $y_r$                          & Parameter f\"{u}r die Ausgangsgr\"{o}{\ss}e f\"{u}r die Konklusion der $r$-ten Regel \\
 $y_{ZR,j}[k]$                  & $k$-ter Abtastzeitpunkt der $j$-ten Zeitreihe der Ausgangsgr\"{o}{\ss}e \\
 $z$                            & 1. interner Zustand eines Neurons,
                                  2. Verschiebungsoperator um einen \newline Abtastzeitpunkt in einer Differenzengleichung\\
 $\mathbf{Z}$                   & Zentriermatrix \\
 $z (t), \mathbf{z} (t)$        & skalare bzw. vektorielle St\"{o}rgr\"{o}{\ss}e eines dynamischen Systems \\
 $Z(z)$                         & $z$-Transformierte der St\"{o}rgr\"{o}{\ss}e $z$ \\
 ZE                             & linguistischer Term Null\\
 ZGF                            & Zugeh\"{o}rigkeitsfunktion \\
 \hline
 \end{tabular}

 \noindent
 \begin{tabular}{|p{.15\textwidth}||p{.79\textwidth}|}
 \hline
 Symbol&Bezeichnung \\ \hline
 ZR                             & Zeitreihe \\
 $\alpha$                       & 1. statistisches Signifikanzniveau f\"{u}r das irrt\"{u}mliche Verwerfen der Nullhypothese,\newline
                                  2. Wichtungsfaktor bzw. Parameter,\newline
                                  3. Frequenzband bei EEG-Daten, \newline
                                  4. Parameter der Diskretisierung von Fuzzy-Mengen ($\alpha$-Schnitt)\\
 $\alpha_i$                     & Wichtungsfaktor f\"{u}r das $i$-te Modell \\
 $\alpha_{krit}$                & Schwellwert \\
 $\alpha_{Imp}$                 & Wichtungsfaktor bez\"{u}glich der Implementierbarkeit \\
 $\alpha_{Int}$                 & Wichtungsfaktor bez\"{u}glich der Interpretierbarkeit \\
 $\beta$                        & 1. statistisches Signifikanzniveau f\"{u}r das irrt\"{u}mliche Verwerfen der Alternativhypothese,\newline
                                  2. Wichtungsfaktor, \newline
                                  3. Frequenzband bei EEG-Daten \\
 $\beta_{Klar}$                 & Wichtungsfaktor f\"{u}r Klarheit \\
 $\beta_l$                      & Parameter eines Cox-Modells \\
 $\beta_{l,i}$                  & Parameter beim Runden von Parametern f\"{u}r Zugeh\"{o}rigkeitsfunktionen\\
 $\gamma$                       & 1. Wichtungsfaktor,
                                  2. Frequenzband bei EEG-Daten \\
 $\delta$                       & Frequenzband bei EEG-Daten \\
 $\delta_c$                     & Wichtungsfaktor bei der Regularisierung f\"{u}r Klasse $c$ \\
 $\Delta \hat{H}$               & Fehlerabsch\"{a}tzungen f\"{u}r Entropie \\
 $\pmb{\varepsilon}$            & Vektor der nicht erkl\"{a}rbaren Reste \\
 $\theta$                       & 1. Parameter bei ROC-Kurven, 2. Frequenzband bei EEG-Daten  \\
 $\pmb{\theta}$                 & Parametervektor \\
 $\Theta$                       & Menge zul\"{a}ssiger Parameter \\
 $\lambda$                      & 1. Eigenwert,
                                  2. Lagrange-Multiplikator\\
 $\Lambda$                      & Likelihood-Quotienten-Kriterium \\
 $\lambda_{sup}$                & Lagrange-Multiplikator eines Support-Vektors\\
 $\mu$                          & 1. Zugeh\"{o}rigkeitswert zu einer Fuzzy-Menge, \newline
                                  2. Frequenzband bei EEG-Daten  \\
 $\mu_A(\cdot)$                 &  Zugeh\"{o}rigkeitsfunktion zu einer Fuzzy-Menge $A$ \\
 $\pmb{\mu}_A(\cdot)$           & Vektor der Zugeh\"{o}rigkeitsfunktionen zu allen linguistischen Termen aller Merkmale\\
 $\pmb{\mu}_{A_l}(\cdot)$       & Vektor der Zugeh\"{o}rigkeitsfunktionen zu allen linguistischen Termen des Merkmals $x_l$ \\
 $\mu_{A_{l,i}}(\cdot)$         & Zugeh\"{o}rigkeitsfunktion zum $i$-ten linguistischen Term des Merkmals $x_l$\\
 $\mu_{A,\alpha}$               & diskretisierte Zugeh\"{o}rigkeitsfunktion bei einem $\alpha$-Schnitt\\
 $\pmb{\mu}_{B}(\cdot)$         & Vektor der Zugeh\"{o}rigkeitsfunktionen zu allen linguistischen Termen der Ausgangsgr\"{o}{\ss}e $y$\\
 $\mu_{B_c}(\cdot)$             & Zugeh\"{o}rigkeitsfunktion zum $c$-ten linguistischen Term der Ausgangsgr\"{o}{\ss}e $y$\\
 $\mu_{B_c,AkI}(\cdot)$         & Zugeh\"{o}rigkeitsfunktion zum $c$-ten linguistischen Term der Ausgangsgr\"{o}{\ss}e $y$ nach der Akkumulation~I \\
 $\mu_{B_c,AkII}(\cdot)$        & Zugeh\"{o}rigkeitsfunktion zum $c$-ten linguistischen Term der Ausgangsgr\"{o}{\ss}e $y$ nach der Akkumulation~II
                                  (Funktion h\"{o}herer Ordnung, Ergebnis ist eine Funktion)\\
 \hline
 \end{tabular}

 \noindent
 \begin{tabular}{|p{.15\textwidth}||p{.79\textwidth}|}
 \hline
 Symbol&Bezeichnung \\ \hline
 $\pmb{\mu}_c$                  & Vektor der Erwartungswerte der Merkmale, in den nur Datentupel der $c$-ten Ausgangsklasse eingehen
                                  (im Abschnitt Statistische Verfahren)\\
 $\mu_n$                        & Lagrange-Multiplikator bei SVMs \\
 $\mu_r$                        & Regelplausibilit\"{a}t \\
 $\mu_{V_r}(\cdot)$             & Zugeh\"{o}rigkeitsfunktion der Pr\"{a}misse der $r$-ten Regel\\
 $\mu_{V_{rl}}(\cdot)$          & Zugeh\"{o}rigkeitsfunktion der $l$-ten Teilpr\"{a}misse der $r$-ten Regel\\
 $\pmb{\mu}_\mathbf{X}$         & Matrix der fuzzifizierten Merkmale ($N$ Zeilen, $\sum_{l=1}^s m_l$ Spalten) \\
 $\pmb{\mu}_{\mathbf{x}_l}$     & Matrix der Zugeh\"{o}rigkeitsgrade zu allen linguistischen Termen des Merkmals $x_l$ f\"{u}r alle $N$ Datentupel\\
 $\pmb{\mu}_\mathbf{y}$         & Matrix der fuzzifizierten Ausgangsgr\"{o}{\ss}e ($N$ Zeilen, $m_y$ Spalten) \\
 $\pmb{\mu}_\mathbf{y}[n,n_{Cl}]$& Vektor der fuzzifizierten Ausgangsgr\"{o}{\ss}e f\"{u}r den Klassifikator $n_{Cl}$ und das $n$-te Datentupel\\
 $\mu_y(y,\mathbf{x})$          & Zugeh\"{o}rigkeitsfunktion nach der Inferenz  (Grad der Empfehlung f\"{u}r verschiedene Werte von $y$) \\
 $\rho, \rho_0, \rho_{i,j}$     & Lernfaktoren \\
 $\xi$                          & Laufvariable f\"{u}r Integrale \\
 $\xi_n$                        & Korrekturwert bei SVMs \\
 $\sigma$                       & Standardabweichung\\
 $\pmb{\Sigma}$              & Kovarianzmatrix der Merkmale\\
 $\sigma^2$                     & Varianz\\
 $\pmb{\Sigma}_c$            & Kovarianzmatrix der Merkmale, in die nur Datentupel der $c$-ten Ausgangsklasse eingehen\\
 $\sigma_l$                     & Standardabweichung des Merkmals $x_l$\\
 $\sigma_{l,Ref}[k]$            & $k$-ter Abtastzeitpunkt der Standardabweichung der $l$-ten Zeitreihe f\"{u}r ein\newline  Referenzkollektiv \\
 $\tau$                         & Laufvariable f\"{u}r die Zeit in einem Integral \\
 $\cup$                         & ODER-Verkn\"{u}pfung\\
 $\cap$                         & UND-Verkn\"{u}pfung\\
 $\| \cdot \|$                  & Norm (allgemein) \\
 $\| \cdot \|_F$                & Frobenius-Norm\\
% \end{supertabular}
\hline
 \end{tabular}
 \end{appendix}
